# Supplementary material for: Quantifying the Prediction Uncertainty of Machine Learning Models for Individual Data
Source: arXiv:2412.07520 source file (2024-12-10)
Supplement: Supplementary file 1 [file appendix.tex]

\chapter{Appendix 1}

appendix 1 content...
